# Supplementary material for: Two-flavor Simulations of the $\rho(770)$ and the Role of the $K\bar K$ Channel
Source: arXiv:1605.04823 ancillary file (2016-08-20)
Supplement: Supplementary file 1 [file supp_3.pdf]

# Supplemental Material for “Two-flavor Simulations of the $\rho(770)$ and the Role of the $K\bar{K}$ Channel”

B. Hu,<sup>1,\*</sup> R. Molina,<sup>1,†</sup> M. Döring,<sup>1,2,‡</sup> and A. Alexandru<sup>1,§</sup>

<sup>1</sup>The George Washington University, Washington, DC 20052, USA

<sup>2</sup>Thomas Jefferson National Accelerator Facility, Newport News, VA 23606, USA

In this supplemental material we present additional graphical representations and tabulated values of the results discussed in the main text. In particular, predicted inelasticities and scattering lengths are compared to experiment, Chiral Perturbation Theory, and a  $N_f = 2 + 1$  lattice simulation. Numerical values for the  $\rho$  masses are tabulated.

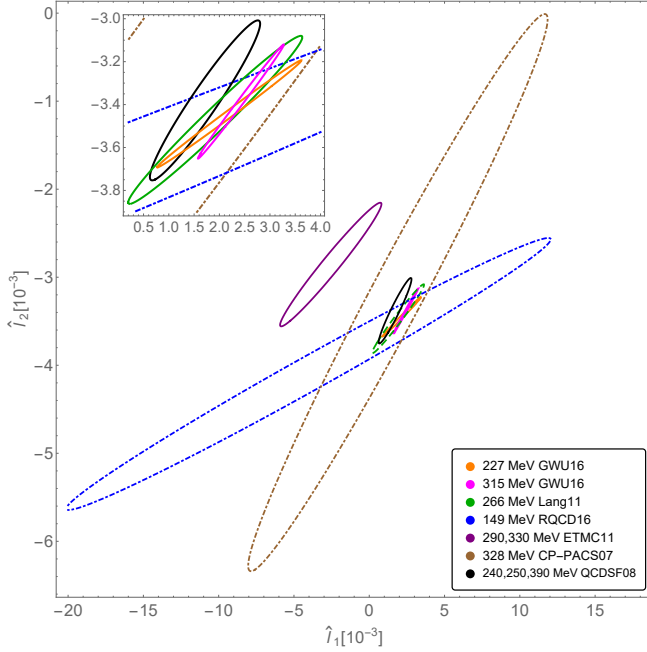

FIG. 1. The 68% confidence error ellipses in  $\hat{l}_1$ ,  $\hat{l}_2$  from fits to the  $N_f = 2$  lattice simulations of Bali *et al.*/RQCD [1], Guo *et al.*/GWU [2], Gökeler *et al.*/QCDSF [5], Lang *et al.* [3], Feng *et al.*/ETMC [6], Aoki *et al.*/CP-PACS [4].

## CONSISTENCY OF FITS

In the main text, the consistency of the fit parameters  $\hat{l}_1$  and  $\hat{l}_2$  is discussed. Fig. 1 displays the 68% confidence error ellipses ( $\Delta\chi^2 = 2.3$ ) from the discussed UCHPT fits to  $N_f = 2$  lattice phase shifts from RQCD [1], GWU [2], Lang *et al.* [3], CP-PACS [4], QCDSF [5] and ETMC [6]. As mentioned in the main text, the error ellipses from RQCD, GWU ( $m_\pi = 227$  MeV and  $m_\pi = 315$  MeV), Lang *et al.*, and CP-PACS all have a common overlap; the ellipse from QCDSF is very slightly off, while the one from ETMC is clearly incompatible.

## MASSES OF THE $\rho$ MESON

In Tab. I we list different values of the  $\rho$  mass. The second column shows the pion masses of the  $N_f = 2$  simulations. At these unphysical masses, the third column indicates the Breit-Wigner  $\rho$  masses as quoted or extracted from plots in the respective publications. The following column shows the Breit-Wigner values converted from our UCHPT fits to the phase shifts: As discussed in the main text, this step is necessary if one decides to quote Breit-Wigner values ( $m_\rho, g$ ) as done here. As expected, the values are very similar to the ones of the third column. The following column “ $N_f = 2$  extrapolated” shows the best fits evaluated at physical pion mass. Note that for the QCDSF and for the ETMC results we fit lattice phase shifts from different pion masses simultaneously as discussed in the main text. The last column shows the outcome after including the  $K\bar{K}$  channel, at the physical pion mass. For these final results we also quote the statistical and systematic uncertainty in parentheses. The latter have been obtained by using different sets of  $\hat{l}_i$  in the  $\pi\pi \rightarrow K\bar{K}$  and  $K\bar{K} \rightarrow K\bar{K}$  transitions as described in the main text.

Fig. 2 illustrates the effect of the  $N_f = 2$  chiral extrapolation indicated with the red arrows. The values before extrapolation correspond to the fourth column of Tab. I, the values after extrapolation to the fifth column. Depending on the used pion masses the values before extrapolation are heavier or lighter than the physical  $\rho$ . After extrapolation the masses are all lighter. The effect of the  $K\bar{K}$  channel is indicated with the black arrows and discussed in the main text. For another way of representing results, see also Fig. 6 of Ref. [2].

## INELASTICITIES AND $K\bar{K}$ PHASE SHIFTS

The observed  $\rho$  mass shift through the  $K\bar{K}$  channel is significant. Therefore, it has to be checked that the  $K\bar{K}$  channel is not in conflict with the observed small inelasticities both in experiment and lattice simulations. In Fig. 3 some results discussed in the main text are illustrated. The upper two rows represent the two-channel ( $\pi\pi$  and  $K\bar{K}$ ) fits to the  $N_f = 2 + 1$  lattice eigenvalues

|               | $M_\pi$ | BW             | BW, converted | $N_f = 2$ extrapolated | $N_f = 2 + 1$ extrapolated |
|---------------|---------|----------------|---------------|------------------------|----------------------------|
| RQCD16 [1]    | 149     | 715(16)(21)    | 714           | 704                    | 770(8)(3)                  |
| GWU16 [2]     | 227     | 749.2(1.6)(15) | 749           | 721                    | 776(3)(10)                 |
|               | 315     | 795.5(0.7)(16) | 795           | 724                    | 778(4)(11)                 |
| QCDSF08 [5]   | 240     | 770            | 776           | 730                    | 779(7)(6)                  |
|               | 250     | 784            | 781           |                        |                            |
|               | 390     | 846            | 844           |                        |                            |
| Lang11 [3]    | 266     | 772(6)(8)      | 774           | 720                    | 776(5)(9)                  |
| ETMC11 [6]    | 290     | 980(31)        | 983           | 821                    | 827(46)(0.4)               |
|               | 330     | 1033(31)       | 1031          |                        |                            |
| CP-PACS07 [4] | 328     | 808(24)(25)    | 833           | 750                    | 786(> 100)(> 100)          |

TABLE I. Breit-Wigner masses of the  $\rho$  meson in MeV. Second column: Pion masses of respective studies [MeV]. Third column: Masses as quoted or extracted from pictures in the respective publications. Fourth column: Breit-Wigner masses  $m_\rho$  (MeV) as reconstructed from our UCHPT solutions at unphysical pion masses. Fifth column: SU(2) extrapolated fits at physical  $M_\pi$ . Sixth column: Final results after including the  $K\bar{K}$  channel. Uncertainties (statistical, systematic) only quoted for these cases.

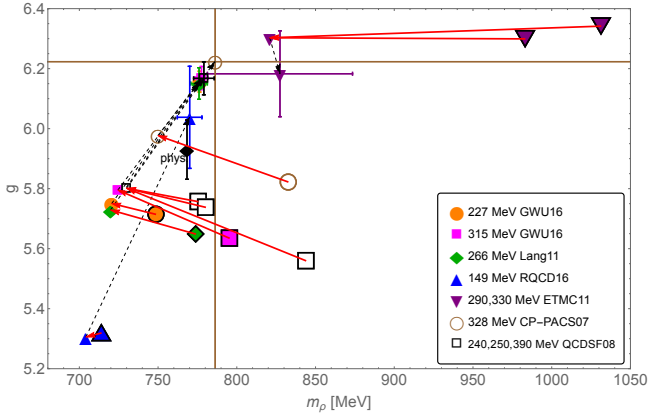

FIG. 2. Effect of the  $N_f = 2$  chiral extrapolation to the physical point in the  $(m_\rho, g)$  plane, indicated with red arrows. The plot markers with black borders stand for unphysical  $(m_\rho, g)$  from Breit-Wigner fits to UCHPT solutions (fourth column of Tab. I). The black arrows are identical to those of Fig. 3 of the main text and indicate the effect of the  $K\bar{K}$  channel. See Fig. 3 of main text for further labeling.

of the HadronSpectrum calculation [7]. The lighter green and gray areas show the results obtained from different analytic fit forms (copied from Fig. 13 of Ref. [7]), the darker areas represent the fit shown in Fig. 11 of Ref. [7]. Additional uncertainties from the conversion to physical units, as done here, are ignored.

We extrapolate our SU(2) fits of the  $N_f = 2$  lattice data to the pion mass of Ref. [7] ( $M_\pi = 236$  MeV). Subsequently, the  $K\bar{K}$  channel ( $M_K = 500$  MeV) is included, taking into account the systematic uncertainties tied to this step as discussed in the main text. This is indicated with the darker red bands in the first two rows of Fig. 3. If on top also statistical uncertainties are included, the areas are indicated with the very narrow lighter red bands around the darker ones. In the figure we only show the case of Lang *et al.* [3] because it is representative for other  $N_f = 2$  lattice simulations, as can be seen from the error

ellipses shown in Fig. 1. We have explicitly checked that the other  $N_f = 2$  data produce similar outcomes for the  $K\bar{K}$  phase shift and inelasticity.

As the figure shows, the predicted  $K\bar{K}$  phase shift is small and with the same negative sign as in the  $N_f = 2+1$  lattice simulation [7] (first row). Also, our predicted inelasticities are in agreement (second row).

Finally, one can also compare to the inelasticity determined from experiment (data points from Ref. [8] in the last row). The latter contains contributions from  $K\bar{K}$  but also from other multi-meson states and provides, thus, only a limit to the present results (red bands). The limits determined in Ref. [11] are even more inelastic. The inelasticity from the  $K\bar{K}$  channel alone, evaluated in Ref. [9] from the Roy-Steiner determination of Ref. [10], is indicated with the black dashed lines. It is indeed of similar, very small, size as our final result.

In addition, the  $K\bar{K}$  inelasticities and  $K\bar{K}$  phase shifts are similarly small as in Ref. [12] (their Fig. 2). Furthermore, we can compare the ratio of couplings at the  $\rho$  resonance pole to the  $\pi\pi$  and the  $K\bar{K}$  channel, recently obtained in the analysis of Ref. [13] (Table I) to be  $R = |g_{\rho \rightarrow K\bar{K}}/g_{\rho \rightarrow \pi\pi}| = 0.64$ . To obtain the corresponding quantity in the present framework, we have selected the global fit solution to experimental scattering, which is characterized by a large shift if the  $K\bar{K}$  channel is removed (see the blue stars in Fig. 3 of the main text). In that property, it is representative for the other results, all exhibiting a substantial shift of the  $\rho$  mass through the  $K\bar{K}$  channel. By analytically continuing this solution to the  $\rho$  pole, we obtain  $R = 0.54$ . In other words, the coupling of the  $\rho$  to the  $K\bar{K}$  channel is even smaller than that in Ref. [13].

## THRESHOLD BEHAVIOR

The predicted scattering lengths and effective ranges are shown in Table II and compared to experiment and the results from Chiral Perturbation Theory of Ref. [14].

|              | Exp./CHPT                                              | RQCD16          | GWU16             |                   | QCDSF08           | Lang11            | ETMC11            | CP-PACS07       |
|--------------|--------------------------------------------------------|-----------------|-------------------|-------------------|-------------------|-------------------|-------------------|-----------------|
|              |                                                        |                 | $m_\pi=227$       | $m_\pi=315$       |                   |                   |                   |                 |
| $10^1 a_1^1$ | <b><math>0.38 \pm 0.02</math></b> (exp.)               | $0.37 \pm 0.31$ | $0.349 \pm 0.003$ | $0.350 \pm 0.001$ | $0.345 \pm 0.003$ | $0.348 \pm 0.005$ | $0.367 \pm 0.003$ | $0.34 \pm 0.67$ |
| $10^2 b_1^1$ | <b><math>0.48</math></b> [ $\mathcal{O}(p^4)$ ]        | $1.14 \pm 29.1$ | $0.638 \pm 0.065$ | $0.627 \pm 0.023$ | $0.695 \pm 0.113$ | $0.656 \pm 0.136$ | $0.911 \pm 0.092$ | $0.701 \pm 40$  |
|              | <b><math>0.79</math></b> [ $\mathcal{O}(p^6)$ , set I] |                 |                   |                   |                   |                   |                   |                 |

TABLE II. Scattering lengths  $a_1^1$  and effective ranges  $b_1^1$  of the final results. Only statistical errors are shown because the systematic ones are very small as expected. The experimental value, the  $\mathcal{O}(p^4)$ , and the  $\mathcal{O}(p^6)$  results are taken from Ref. [14].

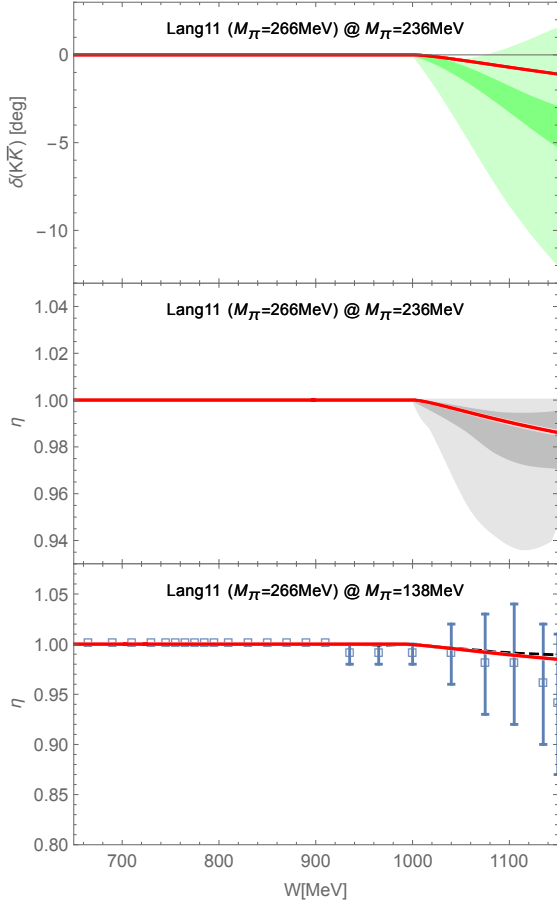

FIG. 3. Upper two rows:  $K\bar{K}$  phase shift and elasticity  $\eta$  at  $M_\pi = 236$  MeV. The green and gray bands show the results of the two-channel fits of Ref. [7] to lattice eigenvalue obtained at this pion mass. The dark red bands show the predictions of this study with systematic uncertainties (very narrow light red bands: statistical uncertainties on top). The last row shows the elasticity at the physical pion mass, together with the elasticity determined from experiment [8] (data points) and the  $K\bar{K}$  contribution to the inelasticity evaluated in Ref. [9] from the Roy-Steiner determination of Ref. [10] (black dashed line).

The lattice data from the GWU, QCDSF, Lang *et al.* and ETMC groups are precise enough to produce relatively small errors. Some scattering lengths are slightly incompatible with the experimental result within the quoted 1- $\sigma$  intervals while the effective ranges are of similar size as the CHPT results.

\* binhu@gwmail.gwu.edu  
† ramope71@email.gwu.edu  
‡ doring@gwu.edu  
§ aalexan@gwu.edu

- [1] G. S. Bali *et al.* [RQCD Collaboration], Phys. Rev. D **93**, 054509 (2016) [arXiv:1512.08678 [hep-lat]].
- [2] D. Guo, A. Alexandru, R. Molina, and M. Döring, arXiv:1605.03993 [hep-lat].
- [3] C. B. Lang, D. Mohler, S. Prelovsek and M. Vidmar, Phys. Rev. D **84**, 054503 (2011); Erratum: [Phys. Rev. D **89**, 059903 (2014)] [arXiv:1105.5636 [hep-lat]].
- [4] S. Aoki *et al.* [CP-PACS Collaboration], Phys. Rev. D **76**, 094506 (2007) [arXiv:0708.3705 [hep-lat]].
- [5] M. Göckeler *et al.* [QCDSF Collaboration], PoS LATTICE **2008**, 136 (2008) [arXiv:0810.5337 [hep-lat]].
- [6] X. Feng, K. Jansen and D. B. Renner, Phys. Rev. D **83**, 094505 (2011) [arXiv:1011.5288 [hep-lat]].
- [7] D. J. Wilson, R. A. Briceño, J. J. Dudek, R. G. Edwards and C. E. Thomas, Phys. Rev. D **92**, 094502 (2015) [arXiv:1507.02599 [hep-ph]].
- [8] S. D. Protopopescu *et al.*, Phys. Rev. D **7**, 1279 (1973).
- [9] F. Niecknig, B. Kubis and S. P. Schneider, Eur. Phys. J. C **72**, 2014 (2012) [arXiv:1203.2501 [hep-ph]].
- [10] P. Büttiker, S. Descotes-Genon and B. Moussallam, Eur. Phys. J. C **33**, 409 (2004) [hep-ph/0310283].
- [11] S. Eidelman and L. Lukaszuk, Phys. Lett. B **582**, 27 (2004) [hep-ph/0311366].
- [12] J. A. Oller, E. Oset and J. R. Pelaez, Phys. Rev. D **59**, 074001 (1999); Erratum: [Phys. Rev. D **60**, 099906 (1999)]; Erratum: [Phys. Rev. D **75**, 099903 (2007)].
- [13] Z. H. Guo and J. A. Oller, Phys. Rev. D **84**, 034005 (2011) [arXiv:1104.2849 [hep-ph]].
- [14] J. Bijnens, G. Colangelo, G. Ecker, J. Gasser and M. E. Sainio, Nucl. Phys. B **508**, 263 (1997) Erratum: [Nucl. Phys. B **517**, 639 (1998)] [hep-ph/9707291].
